# Supplementary material for: Distinct Kondo Screening Behaviors in Heavy Fermion Filled Skutterudites with 4f1 and 4f2 Configurations
Source: arXiv:2006.05093 source file (2020-06-09)
Supplement: Supplementary file 1 [file Skutterudites_supp.pdf]

# Supplementary Material for:

# Distinct Kondo Screening Behaviors in Heavy Fermion Filled Skutterudites with $4f^1$ and $4f^2$ Configurations

X. Lou,[1] H. C. Xu,[1] T. L. Yu,[1] Y. H. Song,[1] C. H. P. Wen,[1] W. Z. Wei,[1] A. Leithe-Jasper,[2] Z. F. Ding,[1] L. Shu,[1,3] S. Kirchner,[4,5] R. Peng,[1,3,*] and D. L. Feng[1,3,6,7,†]

[1]*Laboratory of Advanced Materials, State Key Laboratory of Surface Physics,and Department of Physics, Fudan University, Shanghai 200438, China*

[2]*Max-Planck-Institut für Chemische Physik fester Stoffe, Nöthnitzer Straße 40, 01187 Dresden, Germany*

[3]*Shanghai Research Center for Quantum Sciences, Shanghai 201315, China*

[4]*Zhejiang Institute of Modern Physics and Department of Physics, Zhejiang University, Hangzhou, 310027, China*

[5]*Zhejiang Province Key Laboratory of Quantum Technology and Device, Zhejiang University, Hangzhou 310027, China*

[6]*Collaborative Innovation Center of Advanced Microstructures, Nanjing 210093*

[7]*Hefei National Laboratory for Physical Science at Microscale, CAS Center for Excellence in Quantum Information and Quantum Physics, and Department of Physics, University of Science and Technology of China, Hefei 230026*

## Sec. 1 Method

$CeOs_4Sb_{12}$ (COS) and $PrOs_4Sb_{12}$ (POS) were synthesized by powder metallurgical methods from stoichiometric mixtures of prefabricated $OsSb_2$, $CeSb_2$, $PrSb_2$, and Sb which were compacted and annealed in glassy carbon crucibles sealed into quartz ampoules. (Os-powder, Chempur 99.9 wt. %; Ce, and Pr ingot, AmesLab. 99.9 wt. %; Sb shot, Chempur 99.999 wt. %) Samples were slowly heated to 600°C within 12 hours and annealed for 3 days followed by a regrinding and compacting step with an additional annealing at 800°C for 4 days. Phase purity was checked by powder X-ray diffraction techniques. For crystal growth 5 g of $CeOs_4Sb_{12}$, $PrOs_4Sb_{12}$ powders were blended with 25 g Sb-powder with an addition of 0.1 g $CeSb_2$, or $PrSb_2$, respectively. These mixtures were compacted and placed in a glassy carbon crucible which was then sealed in a quartz ampoule. Crystals were grown by slowly heating up to 900°C within 12 hours with additional soaking time of 12 hours, followed by slow cooling to 600°C within 14 days. Crystals were isolated by sublimation of excess Sb under dynamic vacuum ($10^{-4}$ bar) at 500°C.

High quality single crystals of COS and POS with shining surfaces were

cut into millimeter-scale cubes and aligned by Laue diffraction (See Figs. S1(a)-S1(d)). The samples were notched on the side facets to facilitate cleavage, which gives flat areas significantly larger than the angle-resolved photoemission spectroscopy (APRES) beam spot (See Figs. S1(e)-S1(f)).

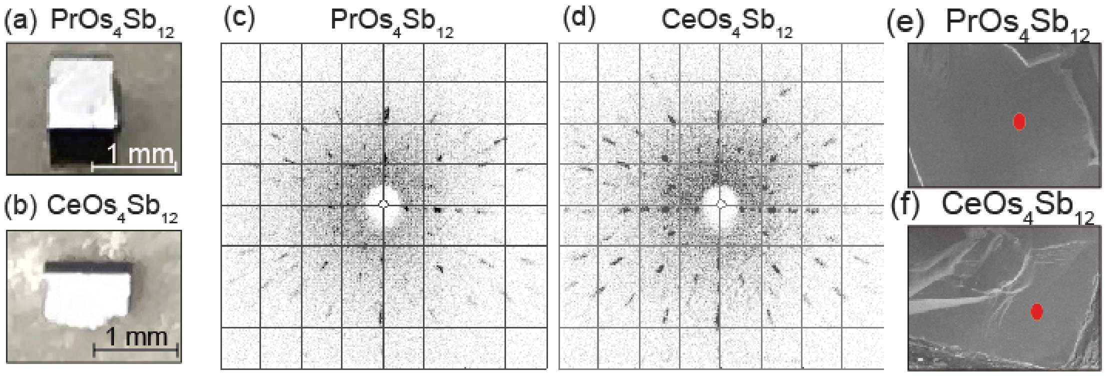


Fig. S1: Optical micrograph of a typical (a) POS and (b) COS samples. Laue pictures of (c) POS and (d) COS. (e) and (f) Scanning electron microscope images of a typical cleaved POS and COS, respectively. ARPES beam spots of 50 μm x 70 μm are illustrated by red filled circles.

The soft X-ray ARPES data were taken at the beamline Advanced Resonant Spectroscopies (ADRESS) of Swiss Light Source (SLS) with the overall energy resolution within 70~150 meV and vacuum ultraviolet APRES studies were conducted at beamline I05 of Diamond Light Source (DLS) and beamline 5-2 of Stanford Synchrotron Radiation Lightsource (SSRL) with overall enenrgy resolution better than 17 meV. The angle resolution for DLS and SSRL is 0.2° while the angle resolution for ADRESS is 0.1°. The samples were cleaved in-situ and measured under a ultra high vacuum better than $1 \times 10^{-10}$ mbar.

## Sec. 2 Surface States

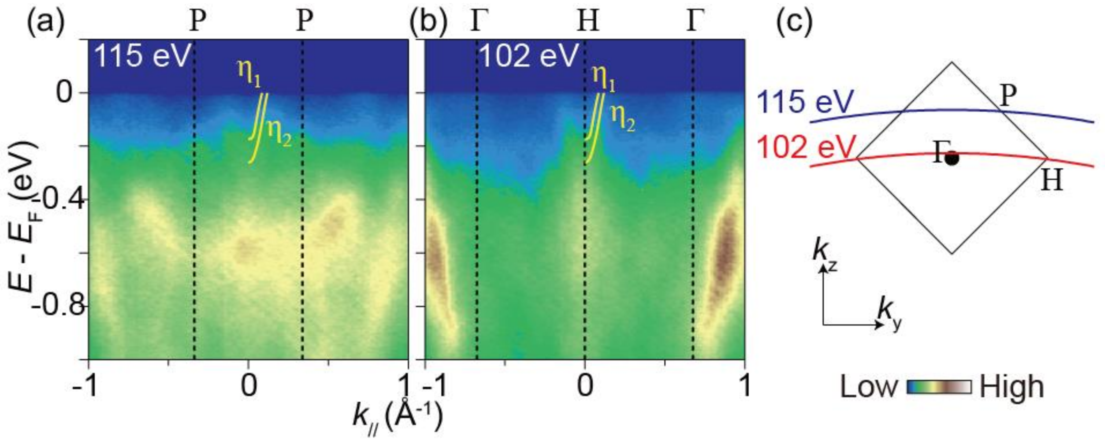


Fig. S2: A comparison of photoemission intensity plot of POS collected with (a) 115 eV and (b) 102 eV. (c) The corresponding positions measured with 115 eV (blue) and 102 eV (red) photons.

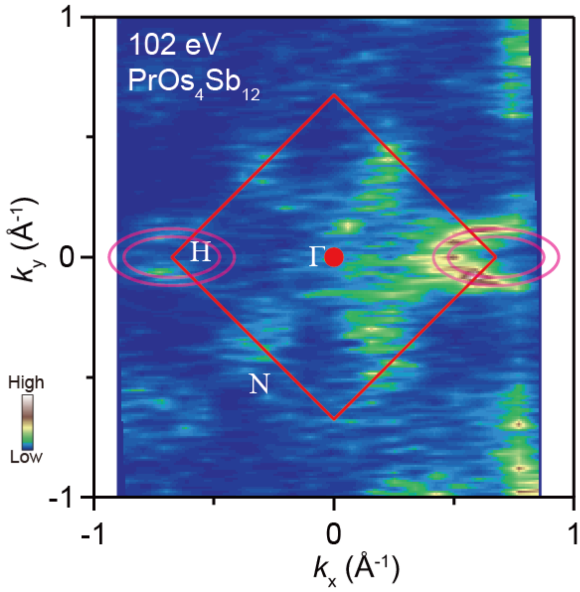


Fig. S3: The Fermi surface map of POS collected with 102 eV photons. Different from the bulk bands showing 4-fold symmetry, the surface states follow the 2-fold symmetry, which is formed by symmetry of the Sb icosahedrons at the cleavage plane.

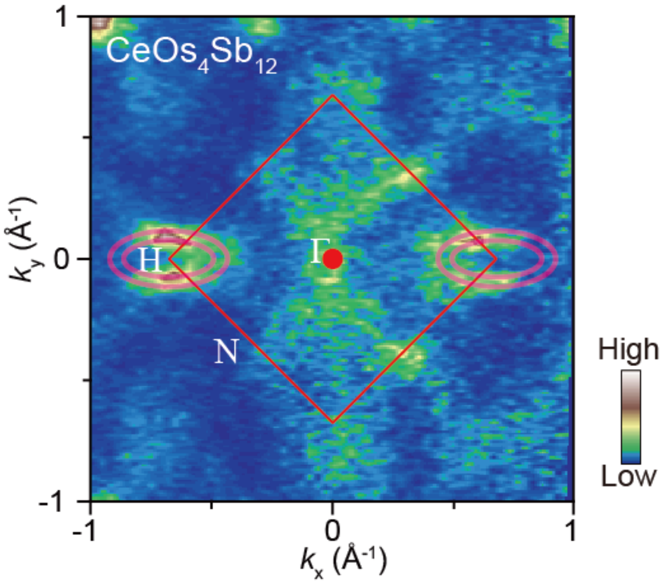


Fig. S4: The Fermi surface map of COS collected with 102 eV photons. Different from the bulk bands showing 4-fold symmetry, the surface states follow the 2-fold symmetry, which is formed by symmetry of the Sb icosahedrons at the cleavage plane.

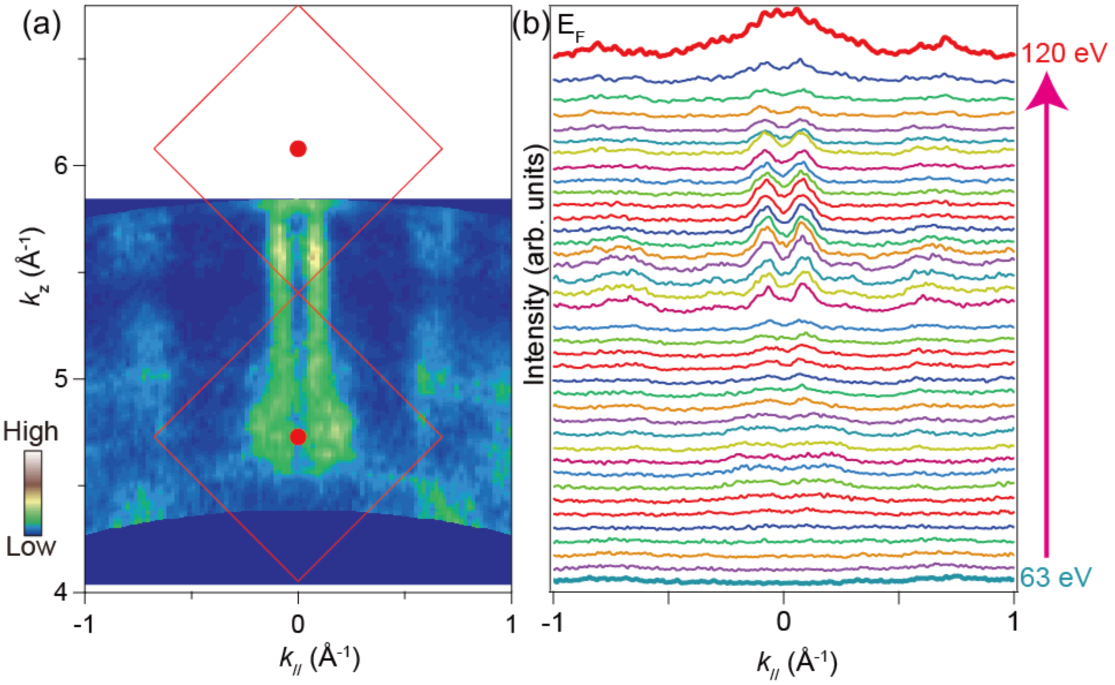


Fig. S5: The Fermi surface map of COS along $k_z$ direction. (b) The corresponding MDCs at Fermi level in (a).

## Sec. 3 X-ray Absorption Spectroscopy (XAS)

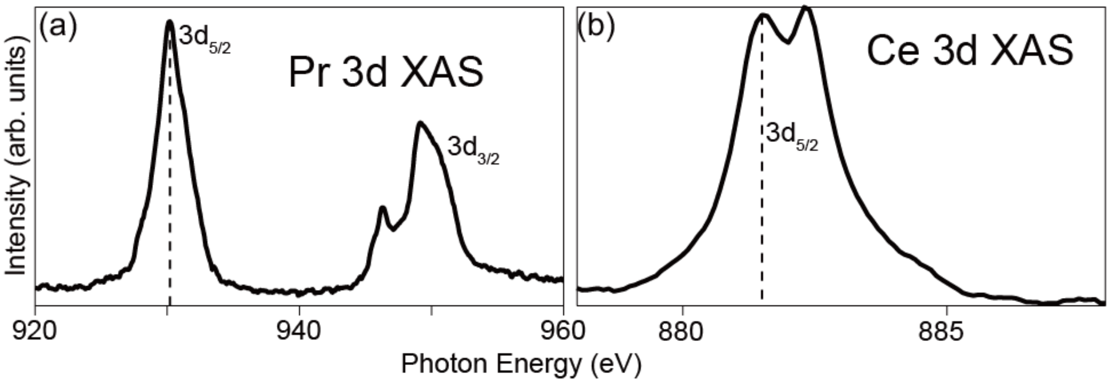


Fig. S6: The XAS of (a) POS and (b) COS. The dashed lines correspond to 930.2 eV for POS and 881.5 eV for COS.

## Sec. 4 Kondo Transition of COS Compared with Other Ce-based Systems

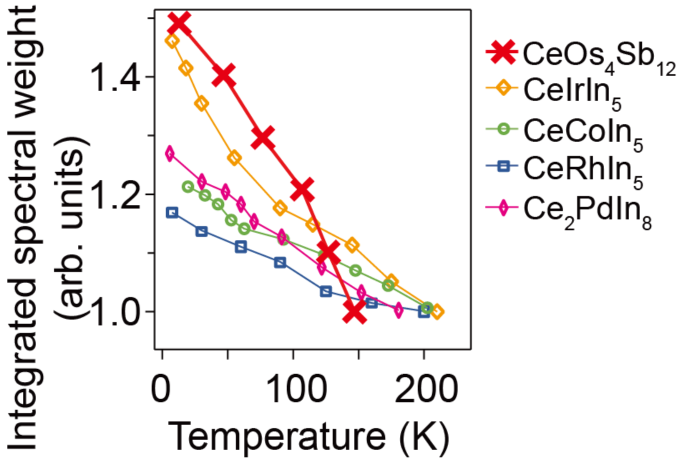


Fig. S7: A comparison of integrated spectral weight in COS, $CeIrIn_5$[1], $CeCoIn_5$[2], $CeRhIn_5$[3] and $Ce_2PdIn_8$[4]. All of data were normalized by the spectral weight at high temperature.

Reference:


[1]. Q. Y. Chen, D. F. Xu, X. H. Niu, J. Jiang, R. Peng, H. C. Xu, C. H. P. Wen, Z. F. Ding, K. Huang, L. Shu, Y. J. Zhang, H. Lee, V. N. Strocov, M. Shi, F. Bisti, T. Schmitt, Y. B. Huang, P. Dudin, X. C. Lai, S. Kirchner, H. Q. Yuan, and D. L. Feng, Phys. Rev. B 96, 045107 (2017).

[2]. Q. Y. Chen, C. H. P.Wen, Q. Yao, K. Huang, Z. F. Ding, L. Shu, X. H. Niu, Y. Zhang, X. C. Lai, Y. B. Huang, G. B. Zhang, S. Kirchner, and D. L. Feng, Physical Review B 97 (2018).

[3]. Q. Y. Chen, D. F. Xu, X. H. Niu, R. Peng, H. C. Xu, C. H. P. Wen, X. Liu, L. Shu, S. Y. Tan, X. C. Lai, Y. J. Zhang, H. Lee, V. N. Strocov, F. Bisti, P. Dudin, J. X. Zhu, H. Q. Yuan, S. Kirchner, and D. L. Feng, Physical Review Letters 120 (2018).

[4]. Q. Yao, D. Kaczorowski, P. Swatek, D. Gnida, C. H. P. Wen, X. H. Niu, R. Peng, H. C. Xu, P. Dudin, S. Kirchner, Q. Y. Chen, D. W. Shen, and D. L. Feng, Physical Review B 99 (2019).
